# Supplementary material for: Prediction of a large-gap and switchable Kane-Mele quantum spin Hall insulator
Source: arXiv:1712.03873 ancillary file (2018-02-19)
Supplement: Supplementary file 1 [file supplementary.pdf]

# Supplemental Material for

# *Prediction of a large-gap and switchable Kane-Mele quantum spin Hall insulator*

Antimo Marrazzo,[1,*] Marco Gibertini,[1] Davide Campi,[1] Nicolas Mounet,[1] and Nicola Marzari[1,†]

[1] *Theory and Simulation of Materials (THEOS) and National Centre for Computational Design and Discovery of Novel Materials (MARVEL), École Polytechnique Fédérale de Lausanne, 1015, Switzerland*

(Dated: February 8, 2018)

## METHODS

### First-principles simulations

DFT calculations are performed using plane waves and pseudopotentials as implemented in the PWscf code of Quantum ESPRESSO distribution [1, 2] in 2D open boundary conditions [3]. The binding energy $E_b$ is computed for the monolayer as extracted from the relaxed 3D bulk, i.e. before DFT structural optimization (relaxation would lower $E_b$ by 3 $\text{meV} \cdot \text{Å}^{-2}$). The interlayer distance and $E_b$ are computed using three different non-local van-der-Waals functionals: the vdW-DF2 functional [4] with C09 exchange (DF2-C09) [5], the revised Vydrov-Van Voorhis (rVV10) functional [6, 7] and the Tkatchenko-Scheffler (TS) functional [8]; we obtain respectively 5.27 Å and 60 $\text{meV} \cdot \text{Å}^{-2}$ with DF2-C09, 5.39 Å and 64 $\text{meV} \cdot \text{Å}^{-2}$ with rVV10, 5.29 Å and 61 $\text{meV} \cdot \text{Å}^{-2}$ with TS, providing a robust agreement for these predictions. We use the Perdew-Burke-Ernzerhof (PBE) [9] functional to study the monolayer, while we added the rVV10 vdW-functional for crystal structure optimization of the BN/$Pt_2HgSe_3$/BN heterostructure. All non-magnetic calculations are performed using ONCV [10] PseudoDojo pseudopotentials [11]; in some cases results are cross-validated using the SSSP pseudopotentials library [12–16]. We test if the monolayer is potentially magnetic by performing three spin-polarized DFT calculations (using the SSSP library v0.7) with random starting magnetization for each species (with an absolute value between 0.1 and 1 $\mu_B \cdot e^{-1}$ and random sign). All calculations end up in the non-spin polarized case with zero magnetization.

$G_0W_0$ calculations are performed using the Yambo [17] code, on top of DFT-PBE calculations with the Quantum ESPRESSO distribution. We use fully relativistic ONCV pseudopotentials from the PseudoDojo library, using the $GW$ version (with complete shell in the valence). The self-energy is constructed using a $36 \times 36 \times 1$ k-point grid; in particular the Green's function is constructed using 1500 bands and the dynamical screening $W$ using 1500 bands and 8 Ry cutoff. In the $G_0W_0$ calculations we adopt the random integration method, 2D Coulomb cutoff and the plasmon pole approximation for the frequency dependence of the self-energy. SOC is included self-consistently at the DFT level, using spin-orbitals, and fully taken into account at the $G_0W_0$ level using a spinorial Green's function. $G_0W_0$ quasi-particle corrections are computed on a $12 \times 12 \times 1$ k-points grid and interpolated using maximally-

localised Wannier functions with WANNIER90 [18]. Topological invariants are computed using Z2pack [20, 21], spectral densities are obtained using WannierTools [22]. Part of the calculations were powered by the AiiDA [23] materials' informatics infrastructure.

**Inversion-symmetry-breaking analysis**

The spacegroup of monolayer Jacutingaite is $P\bar{3}m1$ (164). Inversion symmetry arises from the combination of a 2-fold rotation around an in-plane axis and a reflection through a vertical plane orthogonal to the axis. The loss of inversion symmetry reduces by half the number of symmetries; this can result from either the loss of the rotation or reflection symmetries. In the first case the spacegroup becomes $P3m1$ (156) while in the latter it becomes $P321$ (150). These are the largest subgroups of $P\bar{3}m1$ (164) that lack inversion while keeping all translational symmetries. The transition from $P\bar{3}m1$ (164) to $P3m1$ (156) is driven by atomic displacements that belong to the irreducible representation $A_{2u}$ of the parent group (with the exclusion of a rigid translation along the vertical direction), while the transition from $P\bar{3}m1$ (164) to $P321$ (150) results from atomic displacements belonging to the $A_{1u}$ representation. These are the active representations, while secondary displacements belonging to the trivial $A_{1g}$ representation can always be present as they do not affect the symmetry of the system. In order to assess the nature of atomic displacements, we have projected them onto the possible basis for different irreducible representations of the parent spacegroup $P\bar{3}m1$ (164). There are five different displacement patterns that transform according to the $A_{2u}$ representation (neglecting a trivial translation along the vertical direction), two transforming according to the $A_{1u}$ representation, and three according to the trivial $A_{1g}$ representation that can be obtained using standard group-theory arguments [19]. The unstable phonon mode at $\Gamma$ that appears for calculations without spin-orbit coupling purely belongs to the $A_{2u}$ representation and thus brings the systems towards a more stable phase with spacegroup $P3m1$ (156). The displacements induced by an out-of-plane electric displacement field in the presence of spin-orbit coupling can be instead decomposed into a combination of $A_{1g}$ trivial displacements and $A_{2u}$ displacements that bring the system, also in this case, to the spacegroup $P3m1$ (156). In Fig.3 of the main text we show the amplitude of the atomic displacements projected on the five patterns that transform according to the $A_{2u}$ representation. We point out that the displacement vector in this five-dimensional space

is almost identical for the unstable phonon and the electric-field induced distortion.

## PHONONS

Here we report the phonon dispersions for monolayer Jacutingaite obtained using 2D DFPT [3] with spin-orbit coupling (SOC) and the correct 2D asymptotics [24]. The absence of imaginary frequencies confirms the mechanical stability of the monolayer.

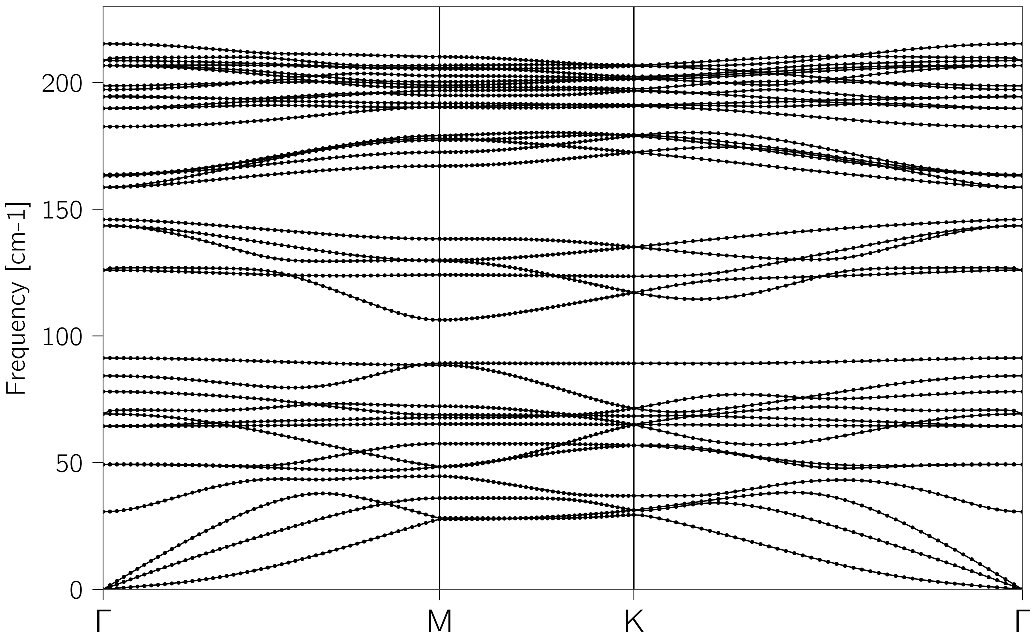


Figure 1. Phonon dispersions of monolayer Jacutingaite obtained using 2D DFPT [3] with spin-orbit coupling (SOC) and the correct 2D asymptotics [24].

## INFRARED AND RAMAN ACTIVE MODES

Here tabulate phonon frequencies at Γ, together with infrared (I) or Raman (R) activity, in order to facilitate the experimental detection of monolayer Jacutingaite through spectroscopic measurements.

| Branch | Frequency [$cm^{-1}$] | Symmetry | Infrared (I) - Raman (R) active |
|---|---|---|---|
| 1-2 | 0.0 | $E_u$ | - |
| 3 | 0.0 | $A_{2u}$ | - |
| 4 | 30.6 | $A_{2u}$ | - |
| 5-6 | 49.3 | $E_u$ | I |
| 7-8 | 64.4 | $E_g$ | R |
| 9-10 | 69.2 | $E_u$ | I |
| 11 | 78.0 | $A_{1g}$ | R |
| 12 | 84.3 | $A_{2u}$ | I |
| 13 | 91.3 | $A_{1u}$ | - |
| 14-15 | 126.0 | $E_u$ | I |
| 16-17 | 143.4 | $E_u$ | I |
| 18 | 146.0 | $A_{2u}$ | I |
| 19-20 | 158.7 | $E_g$ | R |
| 21 | 163.1 | $A_{2g}$ | - |
| 22-23 | 163.7 | $E_g$ | R |
| 24 | 182.6 | $A_{1g}$ | R |
| 25-26 | 189.8 | $E_g$ | R |
| 27-28 | 194.4 | $E_u$ | I |
| 29 | 197.1 | $A_{1g}$ | R |
| 30 | 198.7 | $A_{1u}$ | - |
| 31 | 206.7 | $A_{2u}$ | I |
| 32-33 | 206.7 | $E_u$ | I |
| 34-35 | 208.7 | $E_u$ | I |
| 36 | 215.3 | $A_{2u}$ | I |

Table I. Phonons at Γ, reporting the branch index, the frequency in $cm^{-1}$, the symmetry of the mode, and the mode infrared (I) or Raman (R) activity.

## HEXAGONAL BORON-NITRIDE HETEROSTRUCTURE

Experiments and technological applications of 2D materials inevitably involve a substrate, potentially affecting certain properties. It is thus important to find suitable supporting or encapsulating materials that do not affect the relevant properties of the free-standing monolayer. Here we show how hexagonal boron nitride can encapsulate a monolayer of Jacutingaite and preserve its large-gap QSHI state. Monolayer hexagonal boron nitride (BN) is commensurate to monolayer Jacutingaite ($Pt_2HgSe_3$); they share the same triangular lattice with a BN lattice constant (2.51 Å) three times smaller than monolayer Jacutingaite (7.51 Å). The heterostructure is constructed by creating two identical $3 \times 3$ BN supercells, which are placed above and below the $Pt_2HgSe_3$ monolayer; structural optimization is perfomed using the rVV10 vdW functional [7]. Fig. 2 shows that $Pt_2HgSe_3$ is unaffected by encapsulation, and remains a QSHI, with a band structure near the Fermi level very similar to that of isolated $Pt_2HgSe_3$ monolayer. The BN/$Pt_2HgSe_3$/BN heterostructure is still a QSHI (as confirmed by calculations tracking the hermaphrodite Wannier centres [21]).

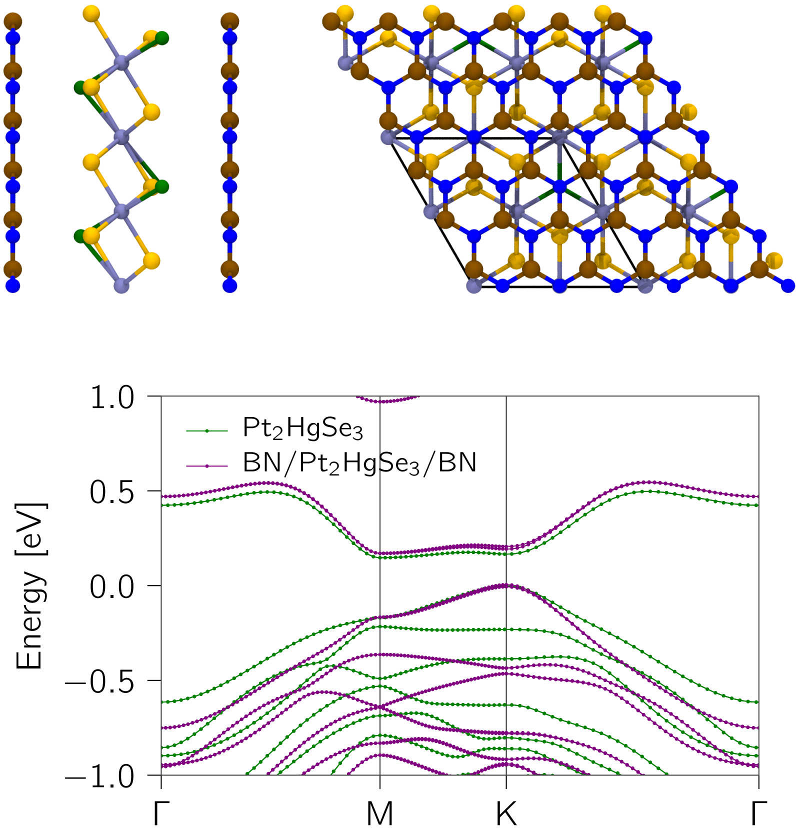


Figure 2. Top panel: side and top view of the relaxed lattice-matched BN/$Pt_2HgSe_3$/BN heterostructure (see text); the unit cell is marked in black. Bottom panel, green: band structure of $Pt_2HgSe_3$ (DFT with SOC). Purple: same for BN/$Pt_2HgSe_3$/BN. It is easily seen that $Pt_2HgSe_3$ is unaffected by encapsulation, and remains a QSHI, with a band structure near the Fermi level very similar to that of isolated $Pt_2HgSe_3$ monolayer (reported in green for reference).

## NANORIBBON

The helical edge states of a QSHI are exponentially localized along the in-plane direction orthogonal to the edges . If the width of a QSHI nanoribbon is comparable or lower than the localization length of the edge states, a gap can be opened by inter-edge interactions. Here we show that 6-cell wide (∼4 nm) nanoribbons are wide enough to completely suppress interactions between the two edges and exhibit gapless helical states as in the semi-infinite-monolayer limit (see Fig. 3).

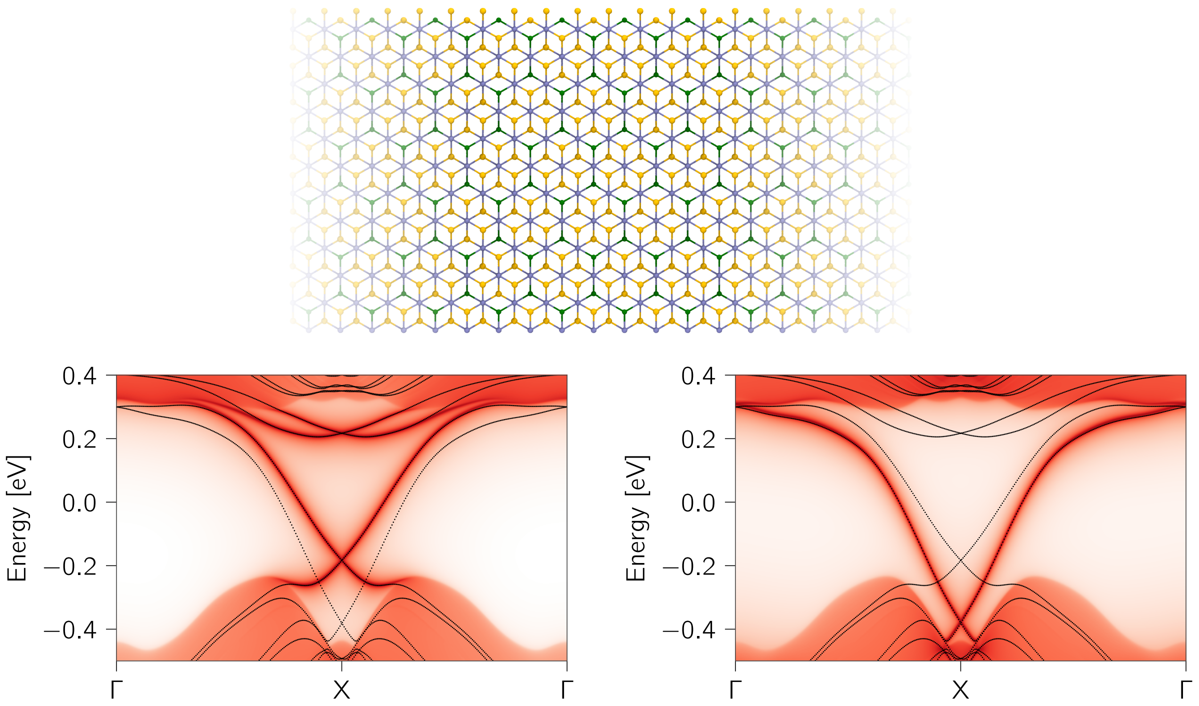


Figure 3. Top panel: zigzag nanoribbon of Jacutingaite, exposing two possible different terminations on the upper and lower edges. Bottom panels: edge spectral densities (red) of a semi-infinite monolayer of Jacuntingaite, with the band structure of 6-cell wide nanoribbons superimposed in black. The two spectral densities (left and right) correspond to the two (lower and upper) possible terminations of the semi-infinite monolayer. The nanoribbon has two pairs of helical states crossing the bulk energy gap, that originate from the lower and upper edges and match perfectly the two corresponding spectral densities of the semi-infinite monolayers. Band structures and spectral densities are obtained with the $G_0W_0$ Wannier Hamiltonian using WANNIER90 [18] and WannierTools [22].

## MODEL HAMILTONIANS

Here we elaborate on how the QSHI phase of monolayer Jacutingaite can be understood in terms of the Kane-Mele model [25, 26], by constructing a tight-binding (TB) model from first principles and comparing it with few different model Hamiltonians. In a buckled honeycomb lattice with time-reversal symmetry, the only tight-binding terms that are allowed up to

second-nearest neighbours are [27]:

$$H = \underbrace{t\sum_{\langle ij\rangle\alpha} c^{\dagger}_{i\alpha}c_{j\alpha}}_{1^{st}\text{NN}} + \underbrace{it_2 \sum_{\langle\langle ij\rangle\rangle\alpha\beta} v_{ij} s^{z}_{\alpha\beta} c^{\dagger}_{i\alpha}c_{j\beta}}_{\text{KM SOC}} + \underbrace{t_2' \sum_{\langle\langle ij\rangle\rangle\alpha} c^{\dagger}_{i\alpha}c_{j\alpha}}_{2^{nd}\text{NN}} + \underbrace{it_2'' \sum_{\langle\langle ij\rangle\rangle\alpha\beta} u_{ij}(\mathbf{s}\times\mathbf{d}^{0}_{ij})^{z}_{\alpha\beta} c^{\dagger}_{i\alpha}c_{j\beta}}_{\text{in-plane SOC}}, \tag{1}$$

where $t, t_2, t_2^{'}$ and $t_2^{''}$ are hopping amplitudes, $v_{ij} = \pm 1$ depending on the orientation of the two nearest-neighbour bonds $\mathbf{d}_{1,2}$ (this can be written as $\mathbf{d}_1 \times \mathbf{d}_2/|\mathbf{d}_1 \times \mathbf{d}_2|$ ), $u_{ij} = \pm 1$ for the two sites and $\mathbf{d}^0_{ij}$ the versor connecting two second nearest neighbours. These four terms represent respectively a real first nearest-neighbour (NN) hopping, the Kane-Mele SOC [25] (second NN), a real second NN hopping and an "in-plane" SOC (second NN). The last term is not present in planar honeycomb lattices such as graphene, but it appears when in-plane mirror symmetry is broken [27]. A first-principles TB Hamiltonian constructed with maximally localised Wannier functions perfectly describes the highest-occupied valence band and lowest unoccupied band (see main text). In Fig.4 we compare the first-principles TB Hamiltonian restricted to first and second NN hoppings with different TB models obtained removing terms from Eq. (1). The Dirac cone due to first NN hoppings is gapped only by the Kane-Mele SOC, while the other terms give negligible or exactly vanishing contributions around K (details in the caption). In fact, a pure Kane-Mele model with first-principles parameters provides a very good description of the low energy physics of monolayer Jacutingaite.

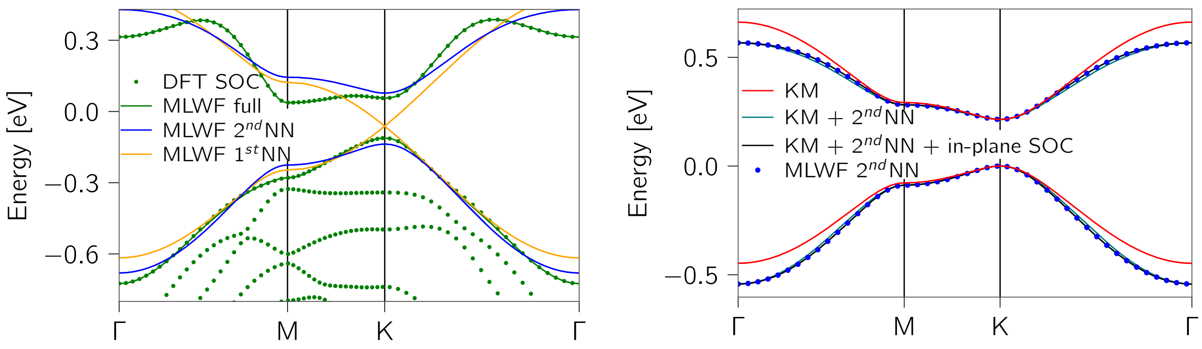


Figure 4. Left panel: band structures obtained from the two-band MLWF DFT SOC Hamiltonian, truncated at various cutoffs. The full MLWF Hamiltonian (green line) perfectly interpolates the highest occupied and lowest unoccupied bands as obtained from a direct DFT calculation (green dots). Truncating the MLWF Hamiltonian to first NN hopping (green line, 6 Å cutoff) turns the gap into a Dirac point; considering second NN hoppings (blue line, 8 Å cutoff) opens a gap at K. Hence, the SOC-induced band gap does not arise from atomic on-site SOC but it is due to the $2^{nd}$ NN hopping term. The second-NN Hamiltonian is sufficient to qualitatively describe the low-energy physics, although further hopping terms slightly renormalize the band gap. Right panel: band structure obtained from different Hamiltonians with parameters extracted from first-principles DFT. A pure KM model (red) correctly describes the band dispersion and the magnitude of the band gap at K. A real second NN hopping term breaks particle-hole symmetry and affects the bands close to Γ, while the bands around K are left unchanged. Owing to the broken planar mirror symmetry of buckled honeycomb lattices, an additional "in-plane" or "intrinsic Rashba" [27] SOC second NN hopping is allowed, exactly vanishing at K and almost negligible all over the high-symmetry path.

## TOPOLOGICAL PHASE DIAGRAM

In monolayer Jacutingaite, robustness and switchability of the QSHI phase coexist thanks to the ionic response. We report the topological phase diagram as a function of the out-of-plane electric displacement field $D_z$ obtained by using a sawtooth potential, disentangling the pure electrostatic contribution from the effect of crystal-symmetry breaking (Fig. 5). We compare the topological phase diagram obtained by freezing the ionic positions in the zero-field configuration or relaxing them. Fig. 5 shows that the ionic distortion greatly reduces the critical field necessary to drive the system into a trivial insulating phase.

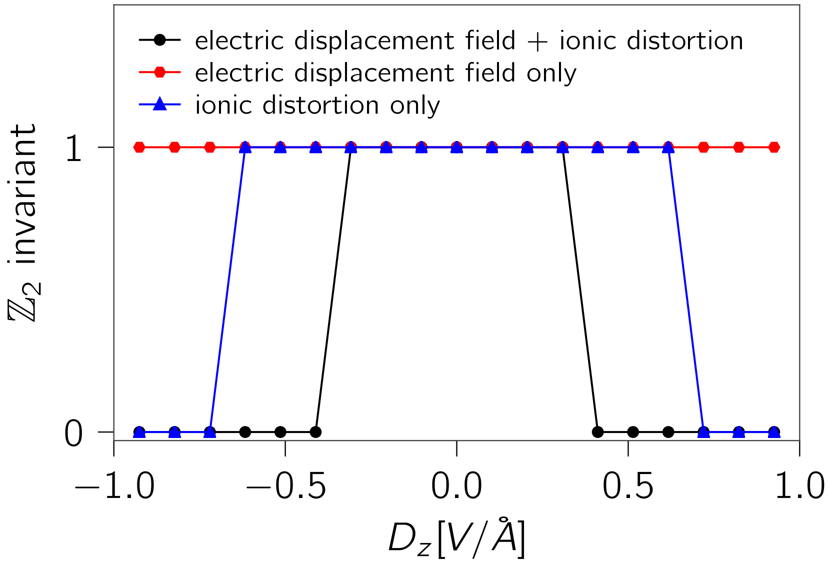


Figure 5. Topological phase diagram: the $\mathbb{Z}_2$ invariant is computed as a function of the out-of-plane electric displacement field $D_z$. The black line represents DFT calculations performed by including self-consistently the electric displacement field $D_z$ and optimizing the ionic position, leading to an ionic distortion as described in the main text. The red line stands for calculations where the electric displacement field is included self-consistently but the ionic positions are kept frozen. Finally, the blue line stands for calculations performed without the electric displacement field but using the ionic positions obtained in the first case. The critical field for the topological phase transition is greatly reduced by the ionic distortion, allowing the cohexistence of large-gap robustness and D-field switchability of the QSHI phase.

## TRACKING OF THE HERMAPHRODITE WANNIER CHARGE CENTRES

Fig. 6 shows the evolution of the hermaphrodite Wannier charge centres (HWCC) [20, 28] and their largest gap for monolayer Jacutingaite, as computed using Z2Pack [21]. The $\mathbb{Z}_2$ invariant can be calculated from the number of HWCC crossing an arbitrary line $x(k)$ across half the BZ: this number modulo two gives the $\mathbb{Z}_2$ invariant, which is one for a QSHI and zero otherwise. For numerical convergence a good choice of $x(k)$ is the largest gap between any two HWCCs at a given $k$ [20, 21].

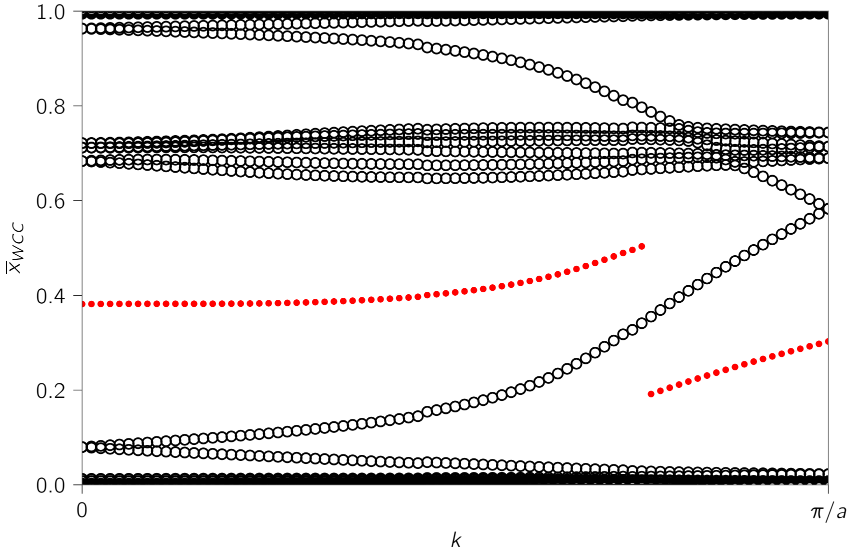


Figure 6. Evolution of the hermaphrodite Wannier centres [20, 28] (circles) of the $G_0W_0$ MLWF Hamiltonian and their largest gap function (red disks), obtained with Z2Pack [21].

## SPIN-ORBIT COUPLING UNRAVELLED

Here we show that the SOC-induced band gap is completely determined by the presence of both Hg and Pt atoms. Fig. 7 shows band structures around the K point obtained by replacing, for one species at a time, the relevant fully-relativistic pseudopotential with its scalar-relativistic version.

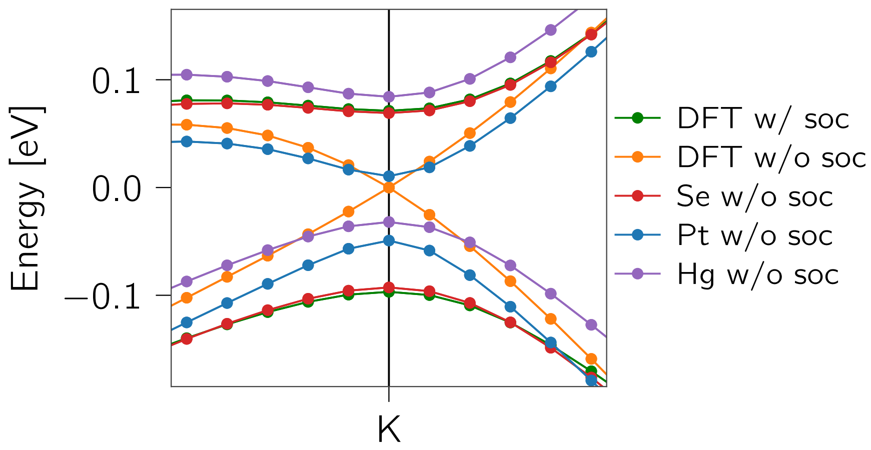


Figure 7. DFT band structure of monolayer Jacutingaite around the K-point, showing the contributions of the different species to the SOC-induced band gap at K, obtained by replacing the relevant fully-relativistic pseudopotential with its scalar-relativistic version. Most of the effects of SOC are due to the presence of Pt atoms (2/3) and Hg atoms (1/3), while Se has little influence on the band gap.

## OXIDATION

Here we study the reactivity of Jacutingaite monolayer against atomic (O) and molecular ($O_2$) oxygen as the most relevant contaminants. DFT energetics indicate that, at zero temperature, $O_2$ is adsorbed to monolayer Jacutingaite and does not dissociate into atomic oxygen. At full $O_2$ coverage, the system is not a QSHI. However, first-principles thermodynamics shows that at room temperature a very moderate vacuum is enough to prevent $O_2$ adsorption.

Calculations are carried out in the unit cell of Jacutingaite and a $2 \times 2$ supercell. The integration over the Brillouin zone is performed with $12 \times 12 \times 1$ and $6 \times 6 \times 1$ k-points grids, respectively. We use norm-conserving, scalar relativistic ONCV [10] PseudoDojo pseudopotentials [11] with a plane wave cutoff of 100 Ry. We check the influence of SOC on the absorption energies only for the lowest energy configurations. In both the atomic and molecular case the effect of SOC on the binding energies turns out to be less than 2%.

### Atomic Oxygen

We first investigate the interaction with a single oxygen atom. The independent lattice sites considered for oxygen adsorption and their naming convention are shown in Fig. 8. Oxygen is put initially in the site and then set free to move. The adsorption energies, defined as $E_{ads}{=}E_{tot} - E_{monolayer} - 1/2N_O E_{O_2}$, are reported in Tab. II. The bridge positions between Se and Pt (B1 and B2) are the most favourable ones with an adsorption energy around 1 eV, followed by the Se top position (T3) with an adsorption energy of 0.67 eV. For combinations of these particular sites we also compute the adsorption energy of two oxygen atoms as might result from the dissociation of an oxygen molecule. Results are reported in Tab. III.

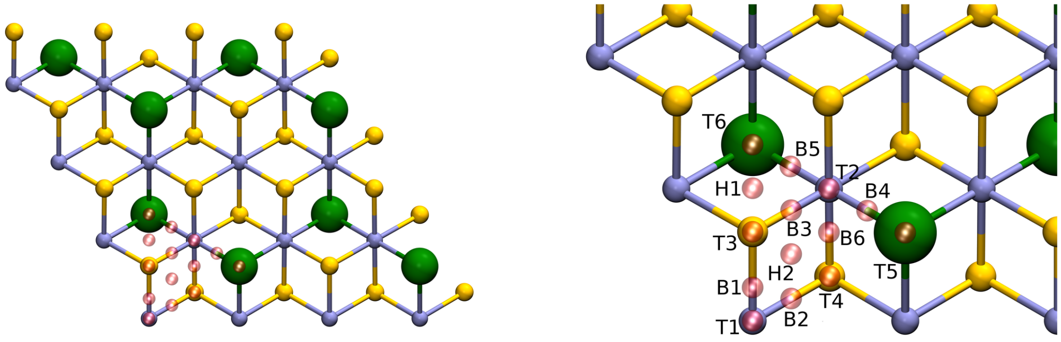


Figure 8. Lattice sites considered for oxygen adsorption on a $2\times2$ supercell (left panel); magnified section (right panel) displaying the sites and the naming convention used in Tab.II

| Adsorption site | Adsorption energy (eV) |
|---|---|
| B1 | -1.01 |
| B2 | -0.97 |
| B3 | -0.81 |
| B4 | +0.26 |
| B5 | +0.75 |
| B6 | -0.81 |
| H1 | -0.27 |
| H2 | -0.42 |
| T1 | +1.80 |
| T2 | +0.25 |
| T3 | -0.67 |
| T4 | -0.45 |
| T5 | +0.70 |
| T6 | +0.30 |

Table II. Adsorption energies for atomic oxygen. The bridge sites between Pt and Se atoms (B1 and B2) and the top site above the Se atom (T3) are the most favourable absorption sites with an adsorption energy of about 1 eV for the former, and 0.67 eV for the latter.

| Adsorption site | Adsorption energy (eV) |
|---|---|
| B1-B2 | -1.62 |
| B1-T3 | -1.97 |
| B2-T3 | -1.53 |
| T3-T3′ | -1.28 |

Table III. Adsorption energy for two oxygen atoms. T3′ indicates an equivalent neighbouring T3 site.

**Molecular oxygen**

Next, we study the interaction of monolayer Jacutingaite with molecular oxygen. As a starting configuration we use molecules with centres having in-plane projections coinciding with the lattice sites considered for atomic adsorption (see Fig. 8). We tested two orthogonal horizontal orientations for the $O_2$ molecule with respect to the monolayer as well as a vertical orientation. All 42 configurations, upon relaxation, evolve into five distinct bound states. The one with the highest adsorption energy (0.77 eV per oxygen molecule) is reported in Fig. 9. In this configuration, one of the atoms in the molecule forms a relatively short bond (2.3 Å) with Hg, while the molecule is slightly elongated by 5%. Almost identical absorption energies are observed for configurations that can be obtained from the one in Fig. 9 applying a rotation around a vertical axis passing through the Hg atom, suggesting a marginal role for the position of the oxygen atom which is farther away from Hg. This adsorption process occurs spontaneously without any activation barrier. The strong hybridization between oxygen $p$ states and Hg states is evident in Fig. 10, showing the band structure of monolayer Jacutingaite after the absorption of a single oxygen molecule in a $2 \times 2$ supercell or in the unit cell. This hybridization is detrimental to the topological order and turns the fully covered system into a trivial insulator. The other four bound states, with considerably lower adsorption energies ranging from 0.1 to 0.3 eV, are reported in Fig. 11.

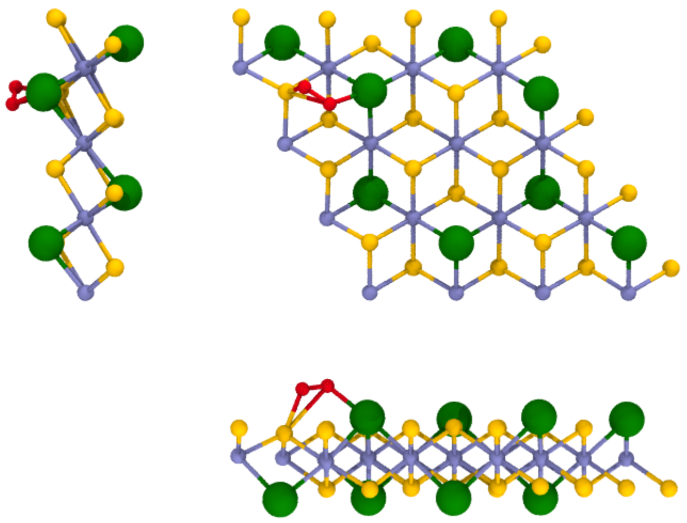

Figure 9. Top and side view of the lowest energy $O_2$ absorption geometry.

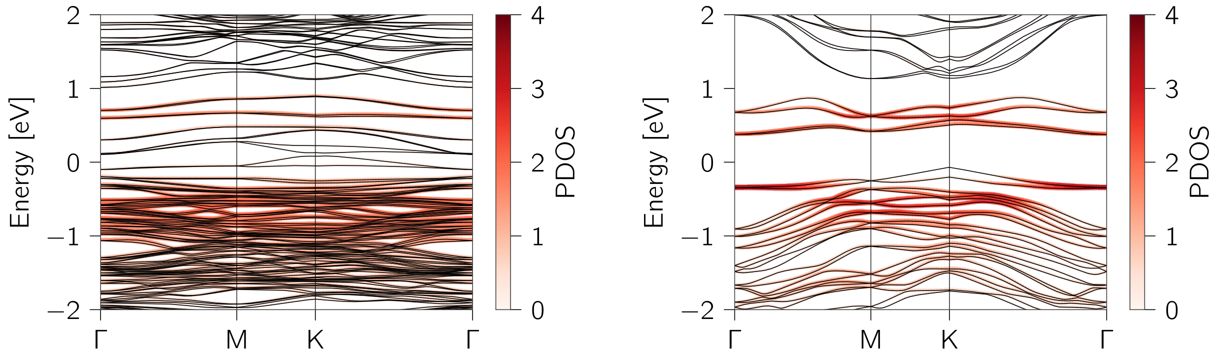


Figure 10. DFT band structure with SOC of $Pt_2HgSe_3$ monolayer after the absorption of a single oxygen molecule in its most stable configuration (see Fig.9) in a $2 \times 2$ supercell (left) and in the unit cell (right). The dot size and color maps the oxygen $p$-orbitals projected density of states; the full band structure is marked by a black line and plotted along the high-symmetry path of the pristine monolayer.

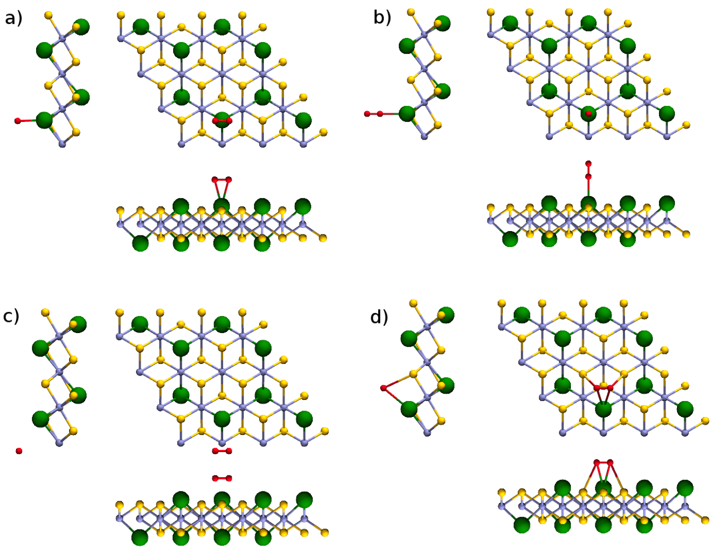


Figure 11. Top and side view of the less favourable $O_2$ adsorption geometries, characterized by adsorption energies of a) 0.15 eV, b) 0.2 eV, c) 0.1 eV and d) 0.32 eV.

### Dissociation of adsorbed molecular oxygen

In order to explore the possibility for a spontaneous dissociation of adsorbed $O_2$ in its lowest energy configuration we carry out climbing-image nudged elastic band (CI-NEB) calculations using a $2 \times 2$ supercell and 8 images. We consider two possible processes, both

starting from the lowest energy $O_2$ adsorption configuration (see Fig.9, or a proper rotational equivalent configuration); one leading to a B1-T3 configuration and the other to a T3-T3′ one. The first dissociation process represent the one with the lowest final energy (with an energy gain of 1.2 eV with respect to the adsorbed molecule), while the second (with an energy gain of only 0.5 eV) is the process that seems most easily accessible since does not require the large structural rearrangement induced by oxygen adsorption in Pt-Se bridge positions. The first process has a large barrier of 2.02 eV while the second a slightly lower one of 1.32 eV. The reaction pathways are reported in Fig.12. Both those values are higher than 0.9 eV, usually taken as threshold under which $O_2$ dissociation can readily happen at ambient condition [29]. We do not compute processes with the configurations B2-T3 and B1-B2 as final states since we believe they present a barrier comparable or higher to the B1-T3 barrier due to the involvement of one or two bridge sites. We can thus conclude that once adsorbed in this configuration $O_2$ is likely to persist in its form.

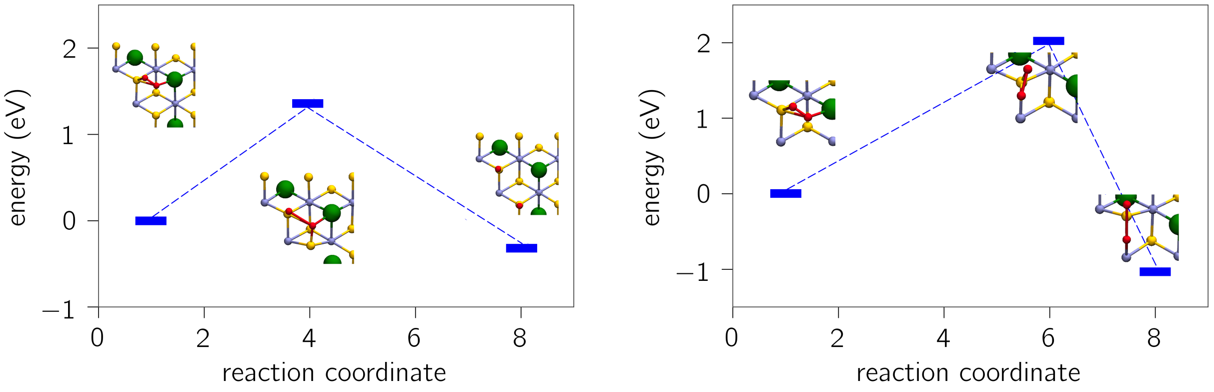


Figure 12. Initial, transition and final states for this $O_2$ molecule as obtained by climbing image NEB adsorbed in the lowest energy configuration, to either dissociate and adsorb in the T3-T3′ configuration (left panel) or the B1-T3 configuration (right panel).

### Thermodynamic effects on molecular adsorption

Since spontaneous $O_2$ dissociation presents such a high activation barrier associative $O_2$ absorption would be the most relevant interaction at ambient conditions. For this reason we study this process in further detail, including thermodynamic effects. Following the first-principles atomistic thermodynamic approach developed in Ref.[30] we study $O_2$ inter-

action as a function of temperature and oxygen partial pressure. The Gibbs free energy of adsorption $\Delta G^{ads}$ is computed as follows:

$$\Delta G^{ads} = E^{ads} + \Delta F^{vib} - \Delta\mu_{O_2}(T, p_{O_2}), \tag{2}$$

where $E^{ads} = E_{2D+O_2} - E_{2D} - E_{O_2}$ is the absorption energy and

$$\Delta\mu_{O_2}(T, p_{O_2}) = \tilde{\mu}_{O_2}(T, p^0) + k_B T \ln\left(\frac{p_{O_2}}{p^0}\right), \tag{3}$$

where $\tilde{\mu}_{O_2}(T, p^0)$ is taken from Ref.[30] and contains all the contributions from vibrations, rotations and ideal gas entropy at 1 atm. We estimate $\Delta F^{vib} = F^{vib}_{2D+O_2} - F^{vib}_{2D}$ by computing the phonons at the $\Gamma$ point and approximating the optical modes as dispersionless phonons. This approximations holds particularly well for vibrations of adsorbed $O_2$, that are the main contributors to $\Delta F^{vib}$.

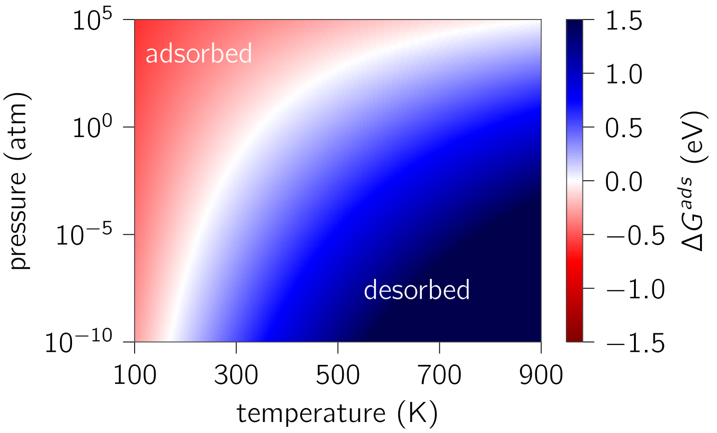


Figure 13. Gibbs free energy of adsorption in eV as a function of oxygen partial pressure and temperature. A negative free energy (red) indicates a tendency to adsorb while a positive free energy (blue) favours desorption.

The behaviour of the Gibbs free energy of adsorption $\Delta G^{ads}$ shows that at room temperature very moderate vacuum is enough to prevent $O_2$ associative adsorption.

## VACANCY FORMATION ENERGIES

Finally we assess the possibility of creating Hg, Pt or Se vacancies by computing the vacancy formation energies for the four inequivalent atoms in monolayer Jacutingaite. The

vacancy formation energy is defined as the difference between the energy of the ideal system and the energy of the defective system plus the energy of the isolated atom. Vacancy formation energies are computed on a $3 \times 3 \times 1$ supercell using scalar-relativistic ONCV [10] PseudoDojo pseudopotentials [11] and 100 Ry cutoff. The results for vacancies in their neutral state and at zero chemical potential are reported in Tab. IV. The Hg vacancy formation energy is the lowest in Jacutingaite and is also rather low when compared to the most common vacancies in other 2D materials like single S or Se vacancies in transition metal dichalcogenides, where formation energies range between 1 and 2 eV depending on the S/Se chemical potential [31–34]. This suggests that particular care should be taken in order to avoid the formation of Hg vacancies during synthesis. However, thanks to the intrinsic robustness of topological properties, moderate amounts of defects—such as Hg vacancies—do not affect the QSHI state.

| Atom | Vacancy formation energy (eV) |
|---|---|
| Hg | 0.50 |
| Pt1 | 12.56 |
| Pt2 | 9.57 |
| Se | 5.27 |

Table IV. Vacancy formation energies. Pt1 represent the platinum atom bonded with Hg while Pt2 is the one bonded with selenium atoms only.

* antimo.marrazzo@epfl.ch
† nicola.marzari@epfl.ch

[1] P. Giannozzi, S. Baroni, N. Bonini, M. Calandra, R. Car, C. Cavazzoni, Davide Ceresoli, G. L. Chiarotti, M. Cococcioni, I. Dabo, A. D. Corso, S. de Gironcoli, S. Fabris, G. Fratesi, R. Gebauer, U. Gerstmann, C. Gougoussis, Anton Kokalj, M. Lazzeri, L. Martin-Samos, N. Marzari, F. Mauri, R. Mazzarello, Stefano Paolini, A. Pasquarello, L. Paulatto, C. Sbraccia, S. Scandolo, G. Sclauzero, A. P. Seitsonen, A. Smogunov, P. Umari, and R. M. Wentzcovitch, Journal of Physics: Condensed Matter **21**, 395502 (2009).

[2] P. Giannozzi, O. Andreussi, T. Brumme, O. Bunau, M. B. Nardelli, M. Calandra, R. Car, C. Cavazzoni, D Ceresoli, M. Cococcioni, N. Colonna, I. Carnimeo, A. D. Corso, S. de Gironcoli, P. Delugas, R. A. D. Jr, A Ferretti, A. Floris, G. Fratesi, G. Fugallo, R. Gebauer, U. Gerstmann, F. Giustino, T. Gorni, J. Jia, M. Kawamura, H-Y Ko, A. Kokalj, E. Küçükbenli, M. Lazzeri, M. Marsili, N. Marzari, F. Mauri, N. L. Nguyen, H.-V. Nguyen, A Otero-de-la-Roza, L. Paulatto, S. Poncé, D. Rocca, R. Sabatini, B. Santra, M. Schlipf, A. P. Seitsonen, A. Smogunov, I Timrov, T. Thonhauser, P. Umari, N. Vast, X. Wu, and S. Baroni, Journal of Physics: Condensed Matter **29**, 465901 (2017).

[3] T. Sohier, M. Calandra, and F. Mauri, Physical Review B **96**, 075448 (2017).

[4] K. Lee, É. D. Murray, L. Kong, B. I. Lundqvist, and D. C. Langreth, Physical Review B **82**, 081101 (2010).

[5] V. R. Cooper, Physical Review B **81**, 161104 (2010).

[6] O. A. Vydrov and T. Van Voorhis, Physical Review Letters **103**, 063004 (2009).

[7] R. Sabatini, T. Gorni, and S. de Gironcoli, Physical Review B **87**, 041108 (2013).

[8] A. Tkatchenko and M. Scheffler, Physical Review Letters **102**, 073005 (2009).

[9] J. P. Perdew, K. Burke, and M. Ernzerhof, Physical Review Letters **77**, 3865 (1996).

[10] D. R. Hamann, Physical Review B **88**, 085117 (2013).

[11] M. J. van Setten, M. Giantomassi, E. Bousquet, M. J. Verstraete, D. R. Hamann, X. Gonze, and G.-M. Rignanese, arXiv:1710.10138 (2017),

[12] G. Prandini, A. Marrazzo, I. Castelli, N. Mounet and N. Marzari, www.materialscloud.org/sssp, in preparation (2018).

[13] K. F. Garrity, J. W. Bennett, K. M. Rabe, and D. Vanderbilt, Computational Materials Science **81**, 446 (2014).

[14] E. Kucukbenli, M. Monni, B. I. Adetunji, X. Ge, G. A. Adebayo, N. Marzari, S. de Gironcoli, and A. D. Corso, arXiv:1404.3015 (2014),

[15] A. Dal Corso, Computational Materials Science **95**, 337 (2014).

[16] M. Schlipf and F. Gygi, Computer Physics Communications **196**, 36 (2015).

[17] A. Marini, C. Hogan, M. Grüning, and D. Varsano, Computer Physics Communications **180**, 1392 (2009).

[18] A. A. Mostofi, J. R. Yates, G. Pizzi, Y.-S. Lee, I. Souza, D. Vanderbilt, and N. Marzari, Computer Physics Communications **185**, 2309 (2014).

[19] ISOTROPY Software Suite, iso.byu.edu.

[20] A. A. Soluyanov and D. Vanderbilt, Physical Review B **83**, 235401 (2011).

[21] D. Gresch, G. Autès, O. V. Yazyev, M. Troyer, D. Vanderbilt, B. A. Bernevig, and A. A. Soluyanov, Physical Review B **95**, 075146 (2017).

[22] Q. Wu, S. Zhang and H-F. Song, M. Troyer and A. A. Soluyanov, Computer Physics Communications **224**, 405 (2018).

[23] G. Pizzi, A. Cepellotti, R. Sabatini, N. Marzari, and B. Kozinsky, Computational Materials Science **111**, 218 (2016).

[24] T. Sohier, M. Gibertini, M. Calandra, F. Mauri, and N. Marzari, Nano Letters **17**, 3758 (2017).

[25] C. L. Kane and E. J. Mele, Physical Review Letters **95**, 226801 (2005).

[26] C. L. Kane and E. J. Mele, Physical Review Letters **95**, 146802 (2005).

[27] C.-C. Liu, H. Jiang, and Y. Yao, Physical Review B **84**, 195430 (2011).

[28] C. Sgiarovello, M. Peressi, and R. Resta, Physical Review B **64**, 115202 (2001).

[29] G. Wang, R. Pandey, and S. P. Karna, WIREs Comput Mol Sci, **7** :e1280 (2017).

[30] K. Reuter and M. Scheffler, Physical Review B **68**, 045407 (2003).

[31] W. Zhou, X. Zou, S. Najmaei, Z. Liu, Y. Shi, J. Kong, J. Lou, P. M. Ajayan, B. I. Yakobson, and J.-C. Idrobo, Nano Letters **13**, 2615 (2013).

[32] H.-P. Komsa and A. V. Krasheninnikov, Physical Review B **91**, 125304 (2015).

[33] J.-Y. Noh, H. Kim, and Y.-S. Kim, Physical Review B **89**, 205417 (2014).

[34] D. Liu, Y. Guo, L. Fang, and J. Robertson, Applied Physics Letters **103**, 183113 (2013).
